# Supplementary material for: Scenic Routes over Points in 2D Space
Source: arXiv:2306.04953 source file (2023-06-08)
Supplement: Supplementary file 1 [file appendix.tex]

\appendix

\section*{Appendix: Pseudocodes}
\label{appendix:a}
Below are the pseudocodes for all the algorithms discussed in Section \ref{sec:algorithms}.

\begin{algorithm}
	\caption{Densest Line Algorithm} 
	\label{alg:densest_line}
	\hspace*{\algorithmicindent} \textbf{Input:} All Pairs Shortest Path $APSP$,  
	\newline
	\hspace*{\algorithmicindent} Number of Lines $K$, Intersection points $I_P$
	\newline
    \hspace*{\algorithmicindent} \textbf{Output:} $K$ Densest Lines.
    
	\begin{algorithmic}[1]
	\State Rank all the bisectors in the bounding box in decreasing order of number of intersection points. Let this ranking be $R$
	\State From $R$, choose the top $K$ bisector lines. Let these lines be $L \subset R$.
	\State For each line in $L$, find its set of endpoints and add them to a set $E$.
	\State Generate an alpha shape on the set $E$.
	\end{algorithmic} 
\end{algorithm}

\begin{algorithm}
	\caption{Min-Max APSP Algorithm} 
	\label{alg:min_max}
	\hspace*{\algorithmicindent} \textbf{Input:} All Pairs Shortest Path $APSP$, Upper Bound $B$, \newline
	\hspace*{\algorithmicindent} Intersection points $I_P$
	\newline
    \hspace*{\algorithmicindent} \textbf{Output:} Subset $S \subset I_P$
    
	\begin{algorithmic}[1]
	\State $S = \phi$
	\State Choose the smallest edge in the graph. Let this edge be between intersection points $(a,b)$
	\State $S = S \cup \{a,b\}$
		\While {$ D \leq B$}
		    \State $D = 0$
		    \State $x = \argmin_{x_i \in (I_P-S)}(\max_{a \in S}(d(x_i,a)))$
		    \State $S = S \cup x_{i}$
		    \State $CH$ = Set of points in Convex Hull of $S$ 
		    \For {$i = 1,\ldots,len(CH)-1$}
		        \State $D \mathrel{{+}{=}} APSP[CH[i]][CH[i+1]]$
		    \EndFor
		\EndWhile
	\end{algorithmic} 
\end{algorithm}

\begin{algorithm}
	\caption{Incremental Expansion Algorithm} 
	\label{alg:triangles}
	\hspace*{\algorithmicindent} \textbf{Input:} All Pairs Shortest Path $APSP$, Upper Bound $B$, \newline
	\hspace*{\algorithmicindent} Intersection points $I_P$
	\newline
    \hspace*{\algorithmicindent} \textbf{Output:} Subset $S \subset I_P$, Outer Edges $E$
    
	\begin{algorithmic}[1]
	\State $S = \phi$, $E = []$
	\State Choose the smallest edge in the graph. Let this edge be between intersection points $(a,b)$
	\State $S = S \cup \{a,b\}$ 
	\newline $E = E.append([a,b])$ 
	\newline $D = d(a,b)$
		\While {$ D \leq B$}
		    \State $X = \phi$
		    \For{$[p,q]$ in $E$}
		        \State $X = X \cup \argmin_{x_i \in (I_P-S)}(d(x_i, p) + d(x_i, q))$
		    \EndFor
		    \If{$len(S) \leq 2$}
		        \State Let $x = X[0]$. \textcolor{gray}{// X only has one element}
		        \State $E.append([a,x], [x,b])$ 
		        \State $D = D + d(a,x) + d(x,b)$
		        \State $S = S \cup \{x\}$
            \Else
                \For{ $[p,q]$ in $E$}
                    \State $x_{c} = \argmin_{x \in X}(d(x,p) + d(x,q) - d(p,q))$
                    \State $p_{c}, q_{c}$ correspond to the chosen p,q above.
                    \State Let $p_c$ be the point closer to $x_c$
                \EndFor
                
                \State $I = [p_c]$ \textcolor{gray}{// Keep track of pts on same line}
                \While{$x_c, p_c, q_c$ all lie on same line}
                    \State $I.append(q_c)$
                    \State $q_c = \argmin_{q \in S-I}(d(x,q))$
                \EndWhile    
                \State $S = S \cup \{x_{c}\}$
                \State \textcolor{gray}{// Delete+Append explained in \ref{ssec:minmax_triangles}}
                \State $E.delete([p_{c}, q_{c}])$ 
                \State $E.append([p_{c}, x_{c}], [x_{c}, q_{c}])$
                \State $D = D + d(p_{c},x_{c}) + d(x_{c},q_{c}) - d(p_{c},q_{c})$
                % \State $CH$ = Set of points in Convex Hull of $S$ 
            \EndIf
		\EndWhile
	\end{algorithmic} 
\end{algorithm}

\begin{algorithm}
	\caption{Endpoints algorithm} 
	\label{alg:endpoints}
	\hspace*{\algorithmicindent} \textbf{Input:} All Pairs Shortest Path $APSP$, Upper Bound $B$, \newline
	\hspace*{\algorithmicindent} Intersection points $I_P$
	\newline
    \hspace*{\algorithmicindent} \textbf{Output:} Subset $S \subset I_P$, Edges $E$
    
	\begin{algorithmic}[1]
	\State $S = \phi$, $E = []$
	\State Choose the smallest edge in the graph. Let this edge be between intersection points $(a,b)$
	\State $S = S \cup \{a,b\}$ 
	\newline $E = E.append([a,b])$ 
	\newline $Endp = \{a,b\}$ \textcolor{gray}{// Endpoints array}
	\newline $D = 0$ \textcolor{gray}{// d(a,b) is APSP distance}
		\While {$ D + d(Endp[0], Endp[1]) \leq B$}
		    \State $x = \argmin_{x_i \in (I_P-S)}(\max_{s \in Endp}(d(x_i,s)))$
		    \State $p = \argmax_{s \in Endp}(d(x,s))$
	        \State $E.append([p,x])$ 
	      %  \State $CH = CH \cup {x}$  
	        \State $S = S \cup {x}$
	        \State $D = D + d(p,x)$
	        \State $Endp = [x, Endp-p]$
		       
		\EndWhile
		\State $E.append(Endp[0], Endp[1])$
		\State $D += d(Endp[0],Endp[1])$
	\end{algorithmic} 
\end{algorithm}
